# Supplementary material for: 2500 vibronic eigenstates of the NO$_3$ radical
Source: arXiv:2407.03398 ancillary file (2024-09-16)
Supplement: Supplementary file 1 [file ESI.pdf]

# Supporting information for: “2500 vibronic eigenstates of the NO<sub>3</sub> radical”

Henrik R. Larsson<sup>1</sup> and Alexandra Viel<sup>2</sup>

<sup>1</sup>*Department of Chemistry and Biochemistry, University of California, Merced, CA 95343, USA*

<sup>2</sup>*Univ. Rennes, CNRS, IPR (Institut de Physique de Rennes) - UMR 6251, F-35000 Rennes, France*

## S1. IR SPECTRA

The dipole moment surface (DMS) from Viel and Eisfeld used in the main text is based on multireference configuration interaction electronic structure wavefunctions.<sup>1</sup> As alternative, we computed a new DMS using the third-order algebraic diagrammatic construction theory for ionization potentials (IP-ADC(3)) using an unrestricted mean-field reference,<sup>2–4</sup> as implemented in the PySCF program package.<sup>5,6</sup> We used the cc-pVTZ basis set<sup>7</sup> and computed integrals using Libcint<sup>8</sup>. The DMS was generated by using Akima-spline-interpolation<sup>9</sup> of a direct-product grid shown in Table S1. Both DMSs are based on the adiabatic electronic ground state. To compute observables for the vibronic states we transformed the DMS to the diabatic representation.

The IR spectrum using the IP-ADC(3)-based DMS is compared to that from Ref. [1] in Fig. S1 (upper and lower panels). Both DMSs lead to a qualitatively similar spectrum with the IP-ADC(3)-based DMS underestimating intensities around 2500 cm<sup>-1</sup>.

The effect of using only Born-Oppenheimer vibrational states is displayed in the middle panel of Fig. S1 using the DMS from Viel and Eisfeld. Many intensities are reduced.

TABLE S1. Coordinate range and number of points used for the construction of the dipole moment surface.

| symbol      | coordinate range | basis size |
|-------------|------------------|------------|
| $\rho$      | [645, 750]       | 13         |
| $\vartheta$ | [0.845, 1.030]   | 8          |
| $\varphi$   | [0.65, 0.88]     | 8          |
| $\theta$    | [1.46, 1.68]     | 9          |
| $\phi$      | [0.88, 1.21]     | 4          |
| $\chi$      | [2.88, 3.45]     | 9          |

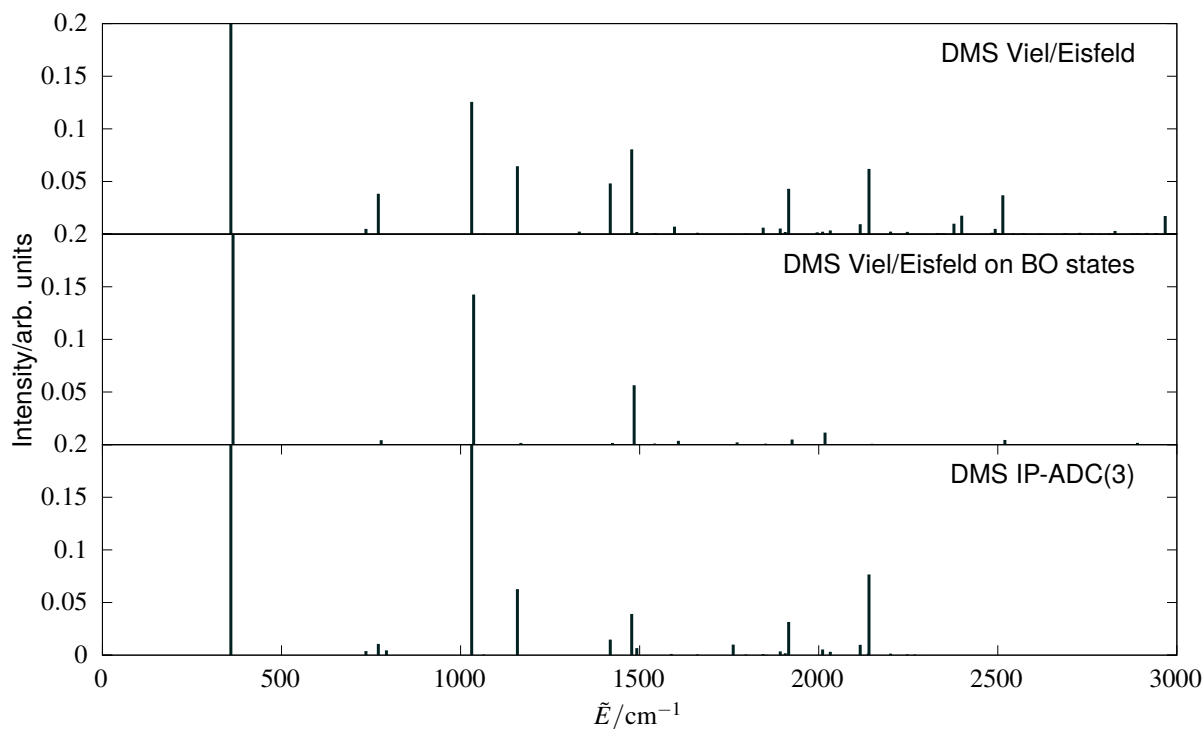

FIG. S1. Computed IR stick spectra. IR spectrum using the dipole moment surface (DMS) from Viel and Eisfeld<sup>1</sup> as found in Fig. 8 in the main text (upper panel), using the same DMS but using the Born-Oppenheimer approximation for the vibrational states (middle panel), and using non-Born-Oppenheimer vibronic states but a DMS computed in this work (lower panel).

- <sup>1</sup>A. Viel and W. Eisfeld, *Chem. Phys.* **509**, 81 (2018).
- <sup>2</sup>J. Schirmer, *Phys. Rev. A* **26**, 2395 (1982).
- <sup>3</sup>A. B. Trofimov and J. Schirmer, *J. Chem. Phys.* **123**, 144115 (2005).
- <sup>4</sup>S. Banerjee and A. Y. Sokolov, *J. Chem. Phys.* **151**, 224112 (2019).
- <sup>5</sup>Q. Sun, T. C. Berkelbach, N. S. Blunt, G. H. Booth, S. Guo, Z. Li, J. Liu, J. D. McClain, E. R. Sayfutyarova, S. Sharma, S. Wouters, and G. K.-L. Chan, *WIREs Comput Mol Sci* **8**, 1340 (2018).
- <sup>6</sup>Q. Sun, X. Zhang, S. Banerjee, P. Bao, M. Barbry, N. S. Blunt, N. A. Bogdanov, G. H. Booth, J. Chen, Z.-H. Cui, J. J. Eriksen, Y. Gao, S. Guo, J. Hermann, M. R. Hermes, K. Koh, P. Koval, S. Lehtola, Z. Li, J. Liu, N. Mardirossian, J. D. McClain, M. Motta, B. Mussard, H. Q. Pham, A. Pulkin, W. Purwanto, P. J. Robinson, E. Ronca, E. R. Sayfutyarova, M. Scheurer, H. F. Schurkus, J. E. T. Smith, C. Sun, S.-N. Sun, S. Upadhyay, L. K. Wagner, X. Wang, A. White, J. D. Whitfield, M. J. Williamson, S. Wouters, J. Yang, J. M. Yu, T. Zhu, T. C. Berkelbach, S. Sharma, A. Y. Sokolov, and G. K.-L. Chan, *J. Chem. Phys.* **153**, 024109 (2020).
- <sup>7</sup>T. H. Dunning, Jr., *J. Chem. Phys.* **90**, 1007 (1989).
- <sup>8</sup>Q. Sun, *J. Comput. Chem.* **36**, 1664 (2015).
- <sup>9</sup>H. Akima, *J. ACM* **17**, 589 (1970).
